# Supplementary material for: Analyzing and Guiding Zero-Shot Posterior Sampling in Diffusion Models
Source: arXiv:2602.07715 source file (2026-05-16)
Supplement: Supplementary file 1 [file Appendix_Posterior_Results.tex]

\section{Posterior Sampling Results}
\begin{table}[H]
\label{sec:Posterior_comparison_results}

  \label{tab:ffhq_lpf_10_sigma_01}
  \centering
  \begin{small}
  \setlength{\tabcolsep}{6pt}
  \begin{tabular}{c c ccc}
  % \begin{sc}
    \toprule
    Method & Steps &
    PSNR$\uparrow$ & SSIM$\uparrow$ & LPIPS$\downarrow$ \\
    \midrule

    \multirow{6}{*}{DPS}
      & 50  & $12.52$ & $0.27$ & $0.69$ \\
      & 100 & $14.99$ & $0.35$ & $0.61$ \\
      & 200 & $18.15$ & $0.44$ & $0.52$ \\
      & 300 & $19.88$ & $0.49$ & $0.48$ \\
      & 400 & $21.04$ & $0.53$ & $0.45$ \\
      & 500 & $21.89$ & $0.55$ & $\mathbf{0.43}$ \\
    \midrule

    \multirow{6}{*}{Spectral}
      & 50  & $\mathbf{16.63}$ & $\mathbf{0.48}$ & $\mathbf{0.60}$ \\
      & 100 & $\underline{17.55}$ & $\underline{0.51}$ & $\mathbf{0.56}$ \\
      & 200 & $\underline{19.01}$ & $\underline{0.53}$ & $\mathbf{0.52}$ \\
      & 300 & $\underline{23.05}$ & $\underline{0.62}$ & $\mathbf{0.43}$ \\
      & 400 & $\underline{23.47}$ & $\underline{0.61}$ & $\underline{0.42}$ \\
      & 500 & $\underline{22.07}$ & $\underline{0.61}$ & $\underline{0.45}$ \\
    \midrule

    \multirow{6}{*}{Spectral $K{=}1$}
      & 50  & $\underline{12.95}$ & $\underline{0.38}$ & $\underline{0.66}$ \\
      & 100 & $\mathbf{18.48}$ & $\mathbf{0.53}$ & $\underline{0.53}$ \\
      & 200 & $\mathbf{22.24}$ & $\mathbf{0.59}$ & $\underline{0.44}$ \\
      & 300 & $\mathbf{23.08}$ & $\underline{0.62}$ & $\mathbf{0.41}$ \\
      & 400 & $\mathbf{24.76}$ & $\mathbf{0.63}$ & $\mathbf{0.39}$ \\
      & 500 & $\mathbf{22.72}$ & $\underline{0.61}$ & $0.44$ \\
    \bottomrule
    % \end{sc}
  \end{tabular}
  \end{small}
\end{table}
